# Supplementary material for: Boosting Novel Category Discovery Over Domains with Soft Contrastive Learning and All-in-One Classifier
Source: arXiv:2211.11262 source file (2023-07-23)
Supplement: Supplementary file 2 [file Sec_appendix_setting_simple.tex]

\subsection{Experimental Setups and Datasets Information}

The compared methods include
two manifold learning methods
(
UMAP \cite{mcinnes_umap_2018} \footnote{https://github.com/lmcinnes/umap},
t-SNE \cite{hinton_reducing_2006} \footnote{https://scikit-learn.org/stable/modules/generated/sklearn.manifold.TSNE.html}
)
and three deep manifold learning methods (
PHATE \cite{moon2019visualizing} \footnote{https://github.com/KrishnaswamyLab/PHATE},
ivis \cite{szubert_structure-preserving_2019} \footnote{https://github.com/beringresearch/ivis} and
parametric UMAP(P-UMAP) \footnote{https://github.com/lmcinnes/umap} \cite{sainburg_parametric_2021}.
)
The datasets include six simple
image datasets (
Digits \footnote{https://scikit-learn.org/stable/auto\_examples/datasets/plot\_digits\_last\_image.html},
Coil20 \footnote{https://www.cs.columbia.edu/CAVE/software/softlib/coil-20.php},
Coil100 \footnote{https://www.cs.columbia.edu/CAVE/software/softlib/coil-100.php},
Mnist \footnote{https://archive.ics.uci.edu/ml/datasets/Optical+Recognition+of+Handwritten+Digits},
EMnist \footnote{https://www.tensorflow.org/datasets/catalog/emnist},
and
KMnist \footnote{https://www.tensorflow.org/datasets/catalog/kmnist}
)
and six biological datasets (
Colon \footnote{https://figshare.com/articles/dataset/The\_microarray\_dataset\_of\_colon\_cancer\_in\_csv\_format\_/13658790/1},
Activity \footnote{https://www.kaggle.com/uciml/human-activity-recognition-with-smartphones} ,
MCA \footnote{https://figshare.com/articles/dataset/MCA\_DGE\_Data/5435866},
Gast10k \footnote{http://biogps.org/dataset/tag/gastric\%20carcinoma/} ,
SAMUSIK \footnote{https://github.com/abbioinfo/CyAnno} ,
and HCL
).

For a fair comparison, we embed the data into a 2-dimensional latent space using the method to be evaluated and then evaluate the method performance by 10-fold cross-validation.
We obtain classification accuracy by applying a linear SVM classifier in the latent space and clustering accuracy by using a kmeans cluster in the latent space.
the classification accuracy and the clustering accuracy are shown in Table \ref{tab:SimpleManifold}
Details of datasets, baseline methods, and evaluation metrics are in the Table \ref{at:5}.

\begin{table*}[h]
  \centering
  \caption{Datasets information of simple manifold embedding task}
  \begin{tabular}{ccc||cccccc}
    \hline
    { Dataset } & { Point Number } & Dimension Number            & { Dataset } & { Point Number } & Dimension Number \\
    \hline
    { Digits }  & { 10,000 }       & { 8$\times$8$\times$1 }     & { Colon }   & { 1,117 }        & { 500 }          \\
    { Coil20 }  & { 1,440 }        & { 128$\times$128$\times$1 } & { Activity} & { 10,299 }       & { 561 }          \\
    { Coil100 } & { 7,200 }        & { 128$\times$128$\times$3 } & { MCA }     & { 30,000 }       & { 34947 }        \\
    { Mnist }   & { 60000 }        & { 28$\times$28$\times$1 }   & { Gast10k } & { 10,638 }       & { 1457 }         \\
    { EMnist }  & { 60000 }        & { 28$\times$28$\times$1 }   & { SAMUSIK } & { 86,864 }       & { 38 }           \\
    { KMnist }  & { 60000 }        & { 28$\times$28$\times$1 }   & { HCL }     & { 60,000 }       & { 27341 }        \\
    \hline
  \end{tabular}
  \label{at:5}
\end{table*}

\subsection{Experimental Parameters}

We use MLP as the network $f_{\theta}$ and network $g_{\phi}$ and use the AdamW optimizer with learning rate 0.001 and weight decay 1e-6.
DLME are trained for 1500 epochs.
The architecture of $f_{\theta}$ is [-1,500,300,80], where -1 mean the dimension of input data.
The architecture of $g_{\phi}$ is [-1,500,80,2].
$\nu_y=100$, and $\alpha = 0.01$.

% We use the grid search to find the best super parameters. 
% The hyperparameters search space are as follows.
% \begin{table}[!htbp]
%   \begin{center}
%   \caption{Hyperparameter search space.}
%   \label{tab:A2}
%   \begin{tabular}{l|c}
%   \hline
%   Hyperparameters & Search Space \\ \hline
%   Data augmentation KNN $K$ & {[}5, 10, 15, 20{]} \\ % \hline
%   degree of freedom in embedding space $\nu^z$ & {[}0.1, 0.01{]} \\ %\hline
%   batch size $\tau$ & {[}300, 3000{]} \\ \hline
%   \end{tabular}
%   \end{center}
%   \end{table}

% The hyperparameters and more information of datasets are shown in table \ref{at:5}.
